# Supplementary material for: Near-Optimal Algorithms for Private Online Optimization in the Realizable Regime
Source: arXiv:2302.14154 source file (2023-02-27)
Supplement: Supplementary file 1 [file appendix-LB.tex]

\section{Proofs for~\cref{sec:lower-bounds}}

\subsection{Proof of~\cref{thm:lb-adaptive-adv}}
\label{sec:apdx-thm-lb-adaptive-adv}

%The upper bound on regret is $\frac{\log d}{\sqrt{n} \diffp}$ and we prove a tight lower bound. 
We build on the following property of the padded Tardos code as done in finger-printing lower bounds.
Given a matrix $X \in \{-1,+1\}^{(n+1) \times p}$, we say that $j \in [p]$ is a consensus column if the column is equal to the all one vector or its negation. Let $X_{(i)} \in \{-1,+1\}^{n \times p}$ denote the matrix that results from removing the $i$'th row in $X$. Moreover, we let $\bar X \in \R^p$ denote the sum of the rows of $X$, that is, $\bar X_j = \sum_{i=1}^{n+1} X_{ij}$. Finally, for $v \in \R^p$ let $\sign(v) \in \{-1,+1\}^p$ denote the signs of the entries of $v$
\begin{theorem}[{\citealp[Theorem 3.2]{TalwarThZh15}}]
\label{thm:lb-fb-matrix}
    Let $p = 1000m^2$ and $n = m/\log m$ for sufficiently large $m$. There exists a matrix $X \in \{-1,+1\}^{(n+1) \times p}$ such that 
    \begin{itemize}
        \item There are at least $0.999p$ consensus columns in $X_{(i)}$
        \item Any algorithm $\A: \{-1,+1\}^{n \times p} \to \{-1,+1\}^p$ such that $\lzero{\A(X_{(i)}) - \mathsf{sign}(\bar X_{(i)})} \le 1/4$ for all $i\in[n+1]$ with probability at least $2/3$ then $\A$ is not $(1,n^{-1.1})$-DP. 
        %with input $X_{(i)}$ for $i \in [n+1]$ such that $\A(X_{(i)})$ produces a $d$-dimensional sign vector which agrees 
    \end{itemize}
\end{theorem}

% \begin{theorem}\cite[theorem 1.1]{SteinkeUl17}
% \label{thm:lb-mean-est}
%     Let $0< \diffp \le 1$ and $\delta \le 1/n^{1+\Omega(1)}$.
%     If $\A : \{-1,+1\}^{n \times d} \to \{-1,+1\}^d$ is \ed-DP then 
%     \begin{equation*}
%       \max_{\Ds} \E \left[ \lone{\A(\Ds) - \bar \Ds} \right] \ge \Omega \left( \frac{d\sqrt{d}}{n \diffp} \right).
%     \end{equation*}
% \end{theorem}

Building on~\cref{thm:lb-fb-matrix}, we can now prove our main lower bound.

\newcommand{\Scons}{S_{\mathsf{cons}}}
\begin{proof}[of \cref{thm:lb-adaptive-adv}]
    First, we prove the lower bound for $\diffp \le 1/(\sqrt{T} \log T)$, that is, we prove the regret has to be linear in this case.
    We will reduce the problem of private sign estimation to DP-OPE with adaptive adversaries and use the lower bound of~\cref{thm:lb-fb-matrix}. To this end, given an algorithm $\A$ for DP-OPE and an input $X \in \{-1,+1\}^{n \times p}$, we have the following procedure for estimating the signs of the columns of $X$. We design an online experts problem that has $d = 2p$ experts where column $j \in [p]$ in $X$ will have two corresponding experts $2j$ and $2j+1$ (corresponding to the sign of column $j$). We initialize the vector of signs $s_j = 0$ for all $1 \le j \le p$. We have $T=0.9p$ rounds and at round $1 \le t \le T$ we sample a user $i_t \sim [n]$ (arbitrarily while enforcing that each $i \in [n]$ appears at most $2T/n$ times) and play a loss function $\ell_t: [d] \to  \{ 0,1 \}$ such that
    \begin{equation*}
        \ell_{t}(2j+1) = 
        \begin{cases}
            1 & \text{if } s_j \neq 0 \\
            \frac{X_{i_t,j}+1}{2} & \text{otherwise}
        \end{cases}
    \end{equation*}
    We also set  
    \begin{equation*}
        \ell_{t}(2j+2) = 
        \begin{cases}
            1 & \text{if } s_j \neq 0 \\
            \frac{-X_{i_t,j}+1}{2} & \text{otherwise}
        \end{cases}
    \end{equation*}
    The idea of this loss function is that the $2j+1$ and $2j+2$ experts will represent the signs of the $j$'th column. If the sign of the $j$'th column is $+1$, then expert $2j+2$ will have better loss and hence should be picked by the algorithm. Moreover, whenever the algorithm has estimated the sign of the $j$'th column ($s_j \neq 0$), we set the loss to be $1$ for both experts $2j+1$ and $2j+2$, in order to force the online algorithm to estimate the sign of new columns. 
    
    Then, given the output of the algorithm $\A$ at time $t$, that is $x_t = \A(\ell_1,\dots,\ell_{t-1})$ we set $s_j = -1$ if $x_{t} = 2j+1$ and $s_j = 1$ if $x_{t} = 2j+2$ and otherwise we keep $s_j$ unchanged. 
    %Note that following this process we will have $s_j \in \{-1,+1\}$ for all $j \in [d]$ after $T=d$ iterations. 
    Moreover, there is an expert that achieves optimal loss, that is, for some $x\opt \in [d]$ we have
    \begin{equation*}
        \sum_{t=1}^T \ell_t(x\opt) = 0.
    \end{equation*}
    This follows since $X$ has at least $0.999p$ consensus columns hence there is a zero-loss expert after $T=0.9p$ iterations. Now we show that if an algorithm $\A$ has small regret, then the vector $s$ estimates the sign of at least $0.8p$ columns. To this end, let $ j_t = \floor{x_t/2}$ denote the column corresponding to the expert picked by the algorithm at time $t$, $S = \{j_t : t \in[T] \}$, and $\Scons = \{ j \in [p]: \text{column j is a consensus column} \} $. Observe that the regret of the algorithm is
    \begin{align*}
        \sum_{t=1}^T \ell_t(x_t) 
        %& =\sum_{t=1}^d \<z_t,e_{j_t} \> \\
        & = \sum_{j_t \in S} \indic{s_{j_t}=1} \ell_t(2j_t+2)
        +  \indic{s_{j_t}=-1} \ell_t(2j_t+1)
        \\ 
        & = \frac{1}{2} \sum_{j_t \in S} \indic{s_{j_t}=1} (-X_{i_t,j_t}+1)
        +  \indic{s_{j_t}=-1} (X_{i_t,j_t}-1) \\
        & = \frac{1}{2} \sum_{j_t \in S} \indic{s_{j_t}=1, X_{i_t,j_t} = -1}
        +  \indic{s_{j_t}=-1, X_{i_t,j_t} = 1} \\
        & = \frac{1}{2} \sum_{j_t \in S} \indic{s_{j_t} \neq X_{i_t,j_t}} \\
        & \ge -0.001 p + \frac{1}{2} \sum_{j_t \in S \cap \Scons} \indic{s_{j_t} \neq X_{i_t,j_t}} \\
        & \ge -0.001 p + \frac{1}{2} \sum_{j_t \in S \cap \Scons} \indic{s_{j_t} \neq \sign(\bar X)_{j_t}}.
        % & = - \sum_{j=1}^d \indic{s_j=1} \Ds_{t,j}
        %   + \sum_{j=1}^d \indic{s_j=-1} \Ds_{t,j} \\
        % & = -\sum_{j=1}^d \indic{s_j = \mathsf{\sign}(\Ds_j)} + \sum_{j=1}^d \indic{s_j \neq \mathsf{\sign}(\Ds_j)} \\
        % & = - d + 2 \lone{s - \bar \Ds}.
    \end{align*}
    Assume towards a contradiction that $\A$ is $(1/200\sqrt{T}\log(T),\delta)$-DP where $\delta \le 1/T^3$ and that the expected regret is at most $T/1000$. Markove inequality implies that with probability at least $9/10$ the regret is at most $T/100$.  Under this event we have
    \begin{equation*}
     \sum_{j_t \in S \cap \Scons} \indic{s_{j_t} \neq \sign(\bar X)_{j_t}} \le 0.002 T.    
    \end{equation*}
    Now note that we can assume that the online algorithm picks $x_t$ such that each $j_t$ appears at most one. Otherwise we can modify the algorithm to satisfy this property while not increasing the regret: whenever the algorithm picks $x_t$ such that $j_t$ appeared before, the loss of this expert is $1$, hence we can randomly pick another expert $x_t$ such that $j_t$ has not appeared. This implies that $|S| = T = 0.9p$ and hence 
    $|S \cap \Scons| \ge 0.85p$. Therefore we have that $s_{j_t} = \sign(\bar X)_{j_t}$ for at least $0.8p$ columns from $\Scons$ with probability $0.9$. To finish the proof, we need to argue about the final privacy guarantee of the sign vector $s$; we will prove that $s$ is $(1,T\delta)$-DP which will give a contradiction to~\cref{thm:lb-fb-matrix} and prove the claim. To this end, note that the algorithm $\A$ is $(1/200\sqrt{T}\log(T),\delta)$-DP. Moreover, recall that each row $i\in[n]$ appears at most $k \le 2T/n \le 2p/n \le 200 \sqrt{p} \log(p)$ times, hence group privacy implies the final output $s$ is $(k\diffp,k\delta)$-DP, that is, $(1,1/T^2)$-DP.
    
    Now we proceed to prove the lower bound for larger values $\diffp \ge 1/(\sqrt{T} \log T)$. Note that if $\diffp \ge \log(T)/T^{1/4}$ then the non-private lower bound of $\sqrt{T \log d}$ is sufficient. Otherwise, consider an algorithm $\A$ that is $\diffp$-DP and consider an adversary that in the first $T_0 < T$ iterations behaves the same as the above where $\diffp = 1/(\sqrt{T_0} \log T_0)$. Then in the last $T - T_0$ iterations it sends $\ell_t(x)=0$ for all $x \in [d]$. The above lower bound implies that the algorithm has to pay regret $\Omega(T_0)= \Omega(1/(\diffp \log T_0)^2)$. The claim follows as $T_0 \le T$.

\end{proof}

\subsection{Proof for~\cref{thm:lb-adaptive-adv-pure}}
\label{sec:proof-lb-pure}

To prove a lower bound for pure DP, we use the following version of~\cref{thm:lb-fb-matrix} for this setting.
\begin{theorem}[{\citealp[Theorem A.1]{SteinkeUl17}}]
\label{thm:pure-sign-est}
    Let $d = 1000n$ and $n$ sufficiently large. Let $\mc{X} = \{X \in \{-1,+1\}^{n \times d} :$ all the columns in $X$ are consensus columns$\} $. Let $\A: \{-1,+1\}^{n \times d} \to \{-1,+1\}^d$ be an algorithm such that for all $X \in \mc{X}$,
    \begin{equation*}
      \E[\lzero{\A(X) - \mathsf{sign}(X)}] \le 1/4.  
    \end{equation*}
     Then $\A$ is not $1$-DP.
\end{theorem}

Using the bound of~\cref{thm:pure-sign-est} and following the same steps as in the proof of~\cref{thm:lb-fb-matrix}, the lower bound of~\cref{thm:lb-adaptive-adv-pure} now follows.

\subsection{Proof of~\cref{thm:lb-large-peps}}
\label{sec:thm-lb-large-peps}

% Idea: Take an $n \times p$ fingerprinting code with $n = \sqrt{p}$ and design experts for every subset of $k$ columns. Now we need $T = p/k$ rounds to estimate all columns.

We use similar ideas to the one in the proof of~\cref{thm:lb-adaptive-adv} where we used a DP-OPE algorithm for sign estimation. Instead of designing two experts for each column, the idea here is to look at subsets of columns of size $k$ and design $2^k$ experts to represent the sign vector of these $k$ columns.

Given an input $X \in \{-1,+1\}^{n \times p}$ where we assume for simplicity that $p/k$ is an integer, we design an expert problem with $d = 2^k \binom{p}{k}  $ experts. %We group the columns into groups of size $k$, that is, $S_i = \{j \in [p] : (i-1)k \le j \le ik\}$ for $i \in [p/k]$. 
Instead of representing the experts as integers $x \in [d]$, we use an equivalent representation where an expert is a pair $(S,v)$ where $S \subset [p]$ is a set of columns of size $k$ and $v \in \{-1,+1\}^k$ represents the signs that this expert assigns for columns in $S$. We initialize the vector of signs $s_j = 0$ for all $1 \le j \le p$.

Here we have $T=0.9p/k$ rounds and at round $1 \le t \le T$ we sample a user $i_t \sim [n]$ (arbitrarily while enforcing that each $i \in [n]$ appears at most $2T/n$ times) and play a loss function $\ell_t$ such that
\begin{equation*}
        \ell_{t}(S,v) = 
        \begin{cases}
            1 & \text{if } s_j \neq 0 \text{ for some } j \in S \\
            0 & \text{otherwise if } \sign(\bar X_S) = v \\
            1 & \text{otherwise}
        \end{cases}
\end{equation*}
 Now, given the output of the algorithm $\A$ at time $t$, that is $x_t = (S_t,v_t)$ we set $s_{S_t} = v_t$ (we assume without loss of generality that each $j \in [p]$ will appear in at most a single $S_t$. Otherwise, similarly to the proof of~\cref{thm:lb-adaptive-adv}, we can ensure this property while not increasing the regret).
    %Note that following this process we will have $s_j \in \{-1,+1\}$ for all $j \in [d]$ after $T=d$ iterations. 
    Moreover, at the end of the game, there is a set $S \subset [p]$ of size $k$ that contains only consensus columns which were not estimated earlier ($S \cap S_t = \emptyset$ for all $t$). This follows from the fact that $X$ has at least $0.999p$ consensus columns hence there is at least $0.05p \ge k$  consensus columns that have not appeared in $S_1,\dots,S_T$, hence there is an expert $(S,v)$ such that 
    \begin{equation*}
        \sum_{t=1}^T \ell_t(S,v) = 0.
    \end{equation*}
    Now we show that if an algorithm $\A$ has small regret, then the vector $s$ estimates the sign of at least $0.8p$ columns. Observe that the regret of the algorithm is
    \begin{align*}
        \sum_{t=1}^T \ell_t(x_t) 
        %& =\sum_{t=1}^d \<z_t,e_{j_t} \> \\
         & = \sum_{t=1}^T  \ell_t(S_t,v_t) 
        \\ 
        & = \sum_{t=1}^T \indic{\sign(\bar X_{S_t}) \neq v_t}
        \\ 
        & = \sum_{t=1}^T \indic{\sign(\bar X_{S_t}) \neq s_{S_t}}.
        %\\ 
        %& \ge -0.001 p +  \sum_{j \in S \cap \Scons} \indic{s_{j} \neq \sign(\bar X)_{j}}.
    \end{align*}
    Assume towards a contradiction that $\A$ is $(\diffp,\delta)$-DP where $\diffp \le  \frac{\sqrt{k/T}}{200\log(T)}$ and $\delta \le 1/T^3$ and that the expected regret is at most $T/1000$. Markov inequality implies that with probability at least $9/10$ the regret is at most $T/100$. %Let $S = \cup_{t=1}^T S_t$ and $\Scons = \{ j \in [p]: \text{column j is a consensus column} \} $. 
    Note that $|S| = kT = 0.9p$.  Under this event we have
    \begin{equation*}
     \sum_{t=1}^T \indic{\sign(\bar X_{S_t}) \neq s_{S_t}}  \le 0.002 T.    
    \end{equation*}
    Hence we have that $\sign(\bar X_{S_t}) = s_{S_t} $ for at least $0.9T$ rounds. As each round has $k$ distinct columns, we have $s_j = \sign(\bar X_j)$ for at least $0.9kT \ge 0.8 p$. As there are at most $0.001p$ non-consensus columns, this means that $s_j = \sign(\bar X_j)$ for at least $0.75p$ consensus columns. Now we prove that $s$ is also $(1,1/T^2)$-DP which gives a contradiction to~\cref{thm:lb-fb-matrix}. To this end, note that the algorithm $\A$ is $(\diffp,\delta)$-DP where $\diffp \le  \frac{\sqrt{k/T}}{200\log(T)} \le  \frac{k/\sqrt{p}}{200 \rho \log(p)} $. Moreover, recall that each row $i\in[n]$ appears at most $k_i \le 2T/n \le 2 p /(nk) \le 200 \sqrt{p} \log(p)/k$ times, hence group privacy implies the final output $s$ is $(\max_{i} k_i \diffp,T \delta)$-DP, that is, $(1,1/T^2)$-DP.
