# Supplementary material for: Near-Optimal Algorithms for Private Online Optimization in the Realizable Regime
Source: arXiv:2302.14154 source file (2023-02-27)
Supplement: Supplementary file 2 [file appendix-oco-imp.tex]

\section{Proofs for~\cref{sec:oco-imp}}

\subsection{Proof of~\cref{sec:thm-oco-imp}}
\label{sec:apdx-thm-oco-imp}

We assume without loss of generality that $L=1$ (otherwise divide the loss by $L$).
As $\mc{X}$ has diameter $D$, we can construct a cover $C = \{c_1,\dots,c_M\}$ of $\mc{X}$ such that $\min_{i \in [M]}\ltwo{x - c_i} \le \rho$ for all $x \in \mc{X}$ where $M \le 2^{d \log(4/\rho)}$~\citep[Lemma 7.6]{Duchi19}. Consider the following algorithm: run~\cref{alg:SD} where the experts are the elements of the cover $C$. \cref{cor:sd-appr} now implies that this algorithm has regret
\begin{equation*}
     \E\left[ \sum_{t=1}^T \ell_t(x_t) - \min_{x \in C} \sum_{t=1}^T \ell_t(x) \right]
     \le O \left( \sqrt{T \ln M } + \frac{T^{1/3} \log^{1/3}(1/\delta) \ln M}{\diffp}  \right).
\end{equation*}
Since $\ell_t$ is $1$-Lipschitz, we now get
\begin{align*}
     \E\left[ \sum_{t=1}^T \ell_t(x_t) - \min_{x \in \mc{X}} \sum_{t=1}^T \ell_t(x) \right]
     & \le \E\left[ \sum_{t=1}^T \ell_t(x_t) - \min_{x \in C} \sum_{t=1}^T \ell_t(x) + \min_{x \in C} \sum_{t=1}^T \ell_t(x)  - \min_{x \in \mc{X}} \sum_{t=1}^T \ell_t(x) \right] \\
     & = O \left( \sqrt{T \ln M } + \frac{T^{1/3} \log^{1/3}(1/\delta) \ln M}{\diffp}  + T\rho \right) \\
     & = O \left( \sqrt{T d \log(1/\rho) } + \frac{T^{1/3} \log^{1/3}(1/\delta) d \log(1/\rho)}{\diffp}  + T\rho \right) \\
     & = O \left( \sqrt{T d \log(T) } + \frac{T^{1/3} d \log^{1/3}(1/\delta)  \log(T)}{\diffp} \right),
\end{align*}
where the last inequality follows by setting $\rho = 1/T$.

\subsection{Proof of~\cref{cor:DP-OCO}}
\label{sec:apdx-cor-DP-OCO}
The algorithm $\Aopt$ is \ed-DP and has excess loss $\Delta_n = LD \cdot O(1/\sqrt{n} + \sqrt{d}/n\diffp)$. Thus, \cref{thm:ub-stoch-OCO} implies that 
\begin{align*}
     \E\left[ \sum_{t=1}^T \ell_t(x_t) - \min_{x \in [d]} \sum_{t=1}^T \ell_t(x) \right]
        & \le \sum_{i=1}^{\log T} 2^i \Delta_i \\
        & \le O(LD) \sum_{i=1}^{\log T} 2^{i/2} + \sqrt{d}/\diffp \\
        & \le LD \cdot O(\sqrt{T} + \sqrt{d} \log(T)/\diffp).
\end{align*}
