# Supplementary material for: Near-Optimal Algorithms for Private Online Optimization in the Realizable Regime
Source: arXiv:2302.14154 source file (2023-02-27)
Supplement: Supplementary file 3 [file appendix-ub.tex]

\section{Proofs for~\cref{sec:ub-obl-sd}}
\label{sec:apdx-ub-obl}

\subsection{Proof of~\cref{thm:ub-priv-DS}}
\label{sec:proof-thm-ub-DS}
We build on the following lemma.
\begin{lemma}
\label{lemma:DS-marg-dist}
    %Let $P_t$ be the marginal distribution of $x_t$ of (non-private) DS algorithm with $z_t \sim \mathsf{Ber}(w^t_{x_{t-1}}/w^{t-1}_{x_{t-1}})$.
    Let $\hat P_t$ be the marginal distribution of $x_t$ of~\cref{alg:SD}. Then 
    \begin{equation*}
        \norm{\hat P_t - P^t}_{TV} \le e^{-Tp/3}.
    \end{equation*}
\end{lemma}
\begin{proof}
    Let $k_t$ be the value of $k$ at iteration $t$. We roughly show that if $k_t < K$ then $P_t = \hat P_t$. As $P(k_t>K)$ is very small, this will prove the claim. Recall that $k_t = \sum_{i \le t} \indic{z_i = 0}$. Note that $P(z_t = 0) \le p + (1-p)\eta \le 2p$. Therefore, letting $y_t \sim \mathsf{Ber}(p + (1-p)\eta)$ we have
    \begin{align*}
    P(k_t > K)
        & \le P(k_T > K) \\
        & = P(\sum_{i=1}^T \indic{z_i = 0}> K) \\
        & \le P(\sum_{i=1}^T \indic{y_i = 0}> K) \\
        & \le e^{-Tp/3},
    \end{align*}
    where the last inequality follows from a Chernoff bound~(\cref{lemma:chernoff}).
    
    Now we proceed to show that $\hat P_t$ and $P_t$ are close. To this end, we first define $Q_t$ to be the marginal distribution of $x_t$ in~\cref{alg:SD} when $K=T+1$ (that is, no limit on switching). We prove by induction that $Q_t = P^t$. The base case for $t=1$ is trivial. Assuming correctness for $t$, we have that for $x \in [d]$
    \begin{align*}
    Q_t(x)  
        & = p p_x^t + (1-p) \frac{w^t_{x}}{w^{t-1}_{x}} Q_{t-1}(x) + (1-p) p_x^t \sum_{x'=1}^d Q_{t-1}(x') (1 - \frac{w^t_{x'}}{w^{t-1}_{x'}}) \\
        & = p p_x^t + (1-p) \frac{w^t_{x}}{w^{t-1}_{x}} \frac{w_x^{t-1}}{W^{t-1}} + (1-p) \frac{w^t_x}{W^t} \sum_{x'=1}^d \frac{w_{x'}^{t-1}}{W^{t-1}}  \frac{w^{t-1}_{x'}-w^t_{x'}}{w^{t-1}_{x'}} \\
        & = p p_x^t + (1-p) \left( \frac{w^t_{x}}{W^{t-1}} +  \frac{w^t_x}{W^t} \frac{W^{t-1} - W^t}{W^{t-1}} \right) \\
        & = p_x^t.
    \end{align*}
    Now consider $\hat P$. Let $Q_t^0$ and $Q_t^1$ be the conditional distribution of $Q_t$ given $k_t<K$ or $k_t \ge K$, respectively.  Moreover, let $\hat P_t^0$ and $\hat P_t^1$ be the conditional distribution of $\hat P_t$ given $k_t<K$ or $k_t \ge K$, respectively. Note that $Q_t(x) =  P(k_t<K) Q_t^0 +  P(k_t<K) Q_t^1$ and that $\hat P_t(x) =  P(k_t<K) \hat P_t^0 +  P(k_t<K) \hat P_t^1$. Noting that $P_t^0 = Q^t_0$, we have
    \begin{align*}
    \norm{\hat P_t - P^t}_{TV}
        & = \norm{\hat P_t - Q^t}_{TV} \\
        & = \norm{P(k_t<K)(\hat P_t^0 - Q_t^0) + P(k_t>K)(\hat P_t^1 - Q_t^1) }_{TV} \\
        & \le  P(k_t<K) \norm{\hat P_t^0 - Q_t^0}  + P(k_t>K) \norm{\hat P_t^1 - Q_t^1}_{TV} \\
        & \le  P(k_t>K).
    \end{align*}
\end{proof}

% \begin{proof}(\cref{lemma:DS-marg-dist})
%     First, note that $z_t \sim \mathsf{Ber}(1-\eta)$ if $\ell_{t-1}(x_{t-1}) = 1$ and otherwise $z_t = 1$.
    
% \end{proof}

\begin{proof}
    First, we begin by analyzing the regret. \cref{lemma:DS-marg-dist} shows that $\hat P_t$ the marginal distribution of $x_t$is the same as that of the (non-private) shrinking dartboard algorithm $P_t$, therefore Theorem 3 of \citet{GeulenVoWi10} shows that for $\eta \le 1/2$
    \begin{align*}
     \E_{x_t \sim \hat P_t}\left[ \sum_{t=1}^T \ell_t(x_t)\right]
        & = \E_{x_t \sim P^t}\left[ \sum_{t=1}^T \ell_t(x_t)\right] 
         +  \E_{x_t \sim \hat P_t}\left[ \sum_{t=1}^T \ell_t(x_t)\right] -  \E_{x_t \sim P^t}\left[ \sum_{t=1}^T \ell_t(x_t)\right] \\
        & \le E_{x_t \sim P^t}\left[ \sum_{t=1}^T \ell_t(x_t)\right]  + 2 T \norm{\hat P_t - P^t}_{TV} \\
        & \le (1+ \eta) \min_{x \in [d]} \sum_{t=1}^T \ell_t(x) + \frac{\ln d}{\eta} + 2 T e^{-Tp/3} \\
        & \le  \min_{x \in [d]} \sum_{t=1}^T \ell_t(x) + \eta T
        + \frac{\ln d}{\eta} + 2 T e^{-Tp/3}. % \\
        %& \le  \min_{x \in [d]} \sum_{t=1}^T \ell_t(x) + \diffp  T^{2/3} 
        %+ \frac{T^{1/3}}{\diffp}  \ln d + 2 T e^{-Tp/3} \\
        %& \le  \min_{x \in [d]} \sum_{t=1}^T \ell_t(x) + \sqrt{T \ln d}
        %+ \frac{T^{1/3}}{\diffp}  \ln d + 2 T e^{-Tp/3},
    \end{align*}

    Let us now analyze privacy. Assume we have two neighboring sequences that differ at time-step $t_1$. 
    Let $Z_t$ and $X_t$ denote the random variables for $z_t$ and $x_t$ in the algorithm when run for the first sequence and let $Y_t = 1 - Z_t$. Similarly, let $Z'_t$, $Y'_t$, and $X'_t$ denote the same for the neighboring sequence. We consider the pairs $W_t = (X_t,Z_{t+1})$ (where $X_0 = 0$) and prove that  $W_t$  given $\{ W_\ell \}_{\ell=0}^{t-1}$ and $W'_t$  given $\{ W'_\ell \}_{\ell=0}^{t-1}$  are $\diffp_t$-indistinguishable where 
    \begin{equation*}
        \diffp_t = 
        \begin{cases}
             0  & \text{if } t < t_1 \\
             \eta/p & \text{if } t = t_1 \\
             \indic{\sum_{\ell=1}^{t-1} Y_\ell < K} 4 Y_t \eta &\text{if } t > t_1
        \end{cases}
    \end{equation*}
    %$\diffp_t = Y_t \eta$ if $\sum_{\ell=1}^{t-1} Y_\ell < K$ and otherwise is $0$-DP (switches are over).
    The result then follows from advanced composition~\citep{DworkRo14}: note that $Y_t \in \{0,1\}$ therefore we have that the final privacy parameter is 
    \begin{align*}
    \diffp_f 
        & \le \frac{3}{2} \sum_{t=1}^T \diffp_t^2 + \sqrt{6 \sum_{t=1}^T \diffp_t^2 \log(1/\delta) } \\
        & \le \frac{3}{2} (\frac{\eta^2}{p^2} + 16 K \eta^2) + \sqrt{6(\frac{\eta^2}{p^2} + 16K \eta^2)\log(1/\delta)  } \\
        & \le  \frac{5\eta}{p} + 24 K \eta^2 + \eta \sqrt{100 K \log(1/\delta)} \\
         & \le  \frac{5\eta}{p} + 100 T p  \eta^2 + 20 \eta \sqrt{ T p \log(1/\delta)}.
    \end{align*}
    Similarly, the result for $\delta=0$ follows from basic composition.
    To finish the proof, consider the pair $W_t$ and $W'_t$. First, note that if $t<t_1$ then clearly $W_t$ and $W'_t$ are $0$-indistinguishable as they do not depend on $\ell_{t_1}$ or $\ell'_{t_1}$. For $t=t_1$, note that $X_{t_1}$ and $X'_{t_1}$ has the same distribution. Moreover, the definition of $Z_t$ implies that 
    $Z_t$ and $Z'_t$ are $\eta/p$-indistinguishable since
    \begin{align*}
    \frac{P(Z_t = 1)}{P(Z'_t = 1)}
        & \le \frac{(1-p)}{(1-p)(1-\eta)} \\
        &  = \frac{1}{1 - \eta} \\
        &  = 1 + \frac{\eta}{1-\eta} \\
        &  \le 1 + 2 \eta \\
        & \le e^{2\eta}. % = e^{2p\diffp}.
    \end{align*}
    Moreover, since $\eta \le p \diffp  $ we have
    \begin{align*}
    \frac{P(Z_t = 0)}{P(Z'_t = 0)}
        & \le \frac{p + (1-p)\eta}{p} \\
        &  \le 1 + \frac{\eta}{p} 
        \le e^{\eta/p}.
    \end{align*}
    Now consider $t>t_1$. If $\sum_{\ell=1}^{t-1} Y_\ell \ge K$ or $Y_t = Y'_t = 0$ then $X_t = X_{t-1}$ and $X'_t = X'_{t-1}$ and thus $X_t$ and $X'_t$ are $0$-indistinguishable.
    If $Y_t = Y'_t = 0$ then $X_t$ and $X'_t$ are $4\eta$-indistinguishable since $w_x^t/w_x^{'t} \le 1/(1-\eta) \le e^{2\eta}$ which implies that $P(x_t = x)/P(x'_t=x) \le e^{4\eta}$. Overall, $X_t$ and $X'_t$ are $4Y_t \eta$-indistinguishable. Moreover, since $t>t_1$, we have that $Z_{t+1}$ is a function of $X_t$ and $\ell_t$  and $Z'_{t+1}$ is a function of $X'_t$ and $\ell'_t=\ell_t$, hence by post-processing we get that $Z_{t+1}$ and $Z'_{t+1}$ are $4Y_t \eta$-indistinguishable. Overall, we have that $W_t$ and $W'_t$ are $\indic{\sum_{\ell=1}^{t-1} Y_\ell < K} 4 Y_t \eta$-indistinguishable.

\end{proof}

\subsection{Proof of~\cref{cor:sd-appr}}
\label{sec:apdx-cor-sd-appr} 
For these parameters, \cref{alg:SD} has privacy
\begin{equation*}
    \diffp_0/4 +  T p^3 \diffp_0^2/4 +  \diffp_0  \sqrt{T p^3\log(1/\delta)} \le 2\diffp_0.
\end{equation*}
As $\diffp_0 \le \diffp/2$, this proves the claim about privacy.
Moreover, its regret is
\begin{align*}
     \eta T
        + \frac{\ln d}{\eta} + 2 T e^{-Tp/3} 
    & \le T p \diffp_0/20 + 20 \ln d /(p\diffp_0) + 2 T e^{-Tp/3} \\
    & \le \frac{T^{2/3} \diffp_0}{\log^{1/3}(1/\delta)} + \frac{20 T^{1/3} \log^{1/3}(1/\delta) \ln d}{\diffp_0} + 2 T e^{-Tp/3} \\
    & \le \sqrt{T \ln d } + \frac{20 T^{1/3} \log^{1/3}(1/\delta) \ln d}{\diffp_0} + 2 T e^{-Tp/3} \\
    & \le O \left(\sqrt{T \ln d } + \frac{ T^{1/3} \log^{1/3}(1/\delta) \ln d}{\diffp} \right),
\end{align*}
where the last inequality follows as $\diffp_0 = \min( \diffp/2,\frac{\log^{1/3}(1/\delta) \sqrt{\ln d}}{T^{1/6}})$.

\subsection{Proof of~\cref{cor:pure}}
\label{sec:apdx-cor-pure} 
For these parameters, \cref{alg:SD} has privacy
\begin{equation*}
    \diffp/20 +  16 Tp \eta 
    \le \diffp/10 +  16Tp^2 \diffp/20
    \le \diffp.
\end{equation*}
Moreover, its regret is
\begin{align*}
     \eta T
        + \frac{\ln d}{\eta} + 2 T e^{-Tp/3} 
    & \le T p \diffp/20 + 20 \ln d /(p\diffp) + 2 T e^{-Tp/3} \\
    & \le \sqrt{T} + \frac{20 \sqrt{T} \ln d}{\diffp} + 2 T e^{-Tp/3},
\end{align*}
where the last inequality follows since $\diffp \le 1$.

\subsection{Proof of~\cref{cor:sd-batch}}
\label{sec:adpx-cor-sd-batch}
\iftoggle{arxiv}{}{
To prove~\cref{cor:sd-batch}, we first prove the following proposition which charactarizes the performance of the private shrinking dartboard algorithm with batches. We prove this result in~\cref{sec:apdx-thm-ub-priv-DS-batch}.
\begin{theorem}
\label{thm:ub-priv-DS-batch}
    %Let $\diffp \le \sqrt{\log d}/T^{1/6}$ and $\delta \le 1$.
    Let $\ell_1,\dots,\ell_T \in [0,1]^d$ be chosen by an oblivious adversary. \cref{alg:SD} with batch size $1 \le B \le T$, $p < 1/2$, $\eta<1/2$, and $K = 2 T p/B $ has regret
    %$p = 1/T^{1/3} < 1/2$, $\eta = p \diffp$, and $K =2 T p $ is $(\diffp_f,\delta)$-DP where $\diffp_f = $ and has regret
    \begin{equation*}
     \E\left[ \sum_{t=1}^T \ell_t(x_t) - \min_{x \in [d]} \sum_{t=1}^T \ell_t(x) \right]
        \le \eta T
        + \frac{B \ln d}{\eta} + 2 T e^{-Tp/3B}.
        %\left(  \frac{\sqrt{T}}{\diffp} \right)^{2/3} \log d \right).
    \end{equation*}
    Moreover, for $\delta>0$, \cref{alg:SD} is $(\diffp,\delta)$-DP where 
    \begin{equation*}
     \diffp = 
          \frac{5\eta}{Bp} + 100 T p  \eta^2/B^3 + \frac{20\eta}{B} \sqrt{12 T p/B \log(1/\delta)}. 
    \end{equation*}
\end{theorem}

We are now ready to prove~\cref{cor:sd-batch}.
}

For these parameters, \cref{alg:SD} has privacy
\begin{equation*}
    \frac{5\eta}{Bp} + \frac{100 T p  \eta^2}{B^3} + \frac{20\eta}{B^{3/2}} \sqrt{ T p \log(1/\delta)} 
    \le \diffp/8 +  \frac{T p^3 \diffp^2}{16B} +   \frac{\diffp}{2} \sqrt{ T p^3 \log(1/\delta)/B} 
    \le \diffp.
\end{equation*}
Moreover, its regret is
\begin{align*}
     \eta T
        + \frac{B\ln d}{\eta} + 2 T e^{-Tp/3B} 
    & \le T B p \diffp/40 + 40 \ln d /(p\diffp) + 2 T e^{-Tp/3B} \\
    & \le \frac{T^{2/3} B^{4/3} \diffp}{\log^{1/3}(1/\delta)} + \frac{40T^{1/3} \log^{1/3}(1/\delta) \ln d}{B^{1/3}\diffp} + 2 T e^{-Tp/3B} \\
    & \le O \left( \frac{T^{2/5} \log^{1/5}(1/\delta) \log^{4/5}(d))  }{\diffp^{4/5}}  + 2 T e^{-Tp/3B} \right),
\end{align*}
where the last inequality follows by choosing $B = \frac{\log^{2/5}(1/\delta) \log^{3/5}(d)}{T^{1/5} \diffp^{3/5}} $ (note that $B \ge 1$ for $\diffp \le  \frac{\log^{2/3}(1/\delta) \log(d)}{T^{1/3}}$) and noticing that $Tp/B \ge \Omega(T^{2/5})$ for these parameters as we have a lower bound on $\diffp$.

\iftoggle{arxiv}{
\subsection{Proof of~\cref{thm:ub-priv-DS-batch}}
\label{sec:apdx-thm-ub-priv-DS-batch}
}{
\subsection{Proof of~\cref{thm:ub-priv-DS-batch}}
\label{sec:apdx-thm-ub-priv-DS-batch}
}
    The same analysis as in~\cref{thm:ub-priv-DS} yields regret
    \begin{equation*}
     \E\left[ \sum_{t=1}^{\tilde T} \tilde \ell_t(\tilde x_t) - \min_{x \in [d]} \sum_{t=1}^T \tilde  \ell_t(x) \right]
        \le \eta \tilde T
        + \frac{\ln d}{\eta} + 2 \tilde  T e^{-\tilde Tp/3}.
        %\left(  \frac{\sqrt{T}}{\diffp} \right)^{2/3} \log d \right).
    \end{equation*}
    Setting $x_t = \tilde x_{\floor{t/B}}$ and multiplying both sides by $B$, we have regret
    \begin{equation*}
     \E\left[ \sum_{t=1}^{ T}  \ell_t(x_t) - \min_{x \in [d]} \sum_{t=1}^T  \ell_t(x) \right]
        \le \eta  T
        + \frac{B \ln d}{\eta} + 2  T e^{-\tilde Tp/3}.
        %\left(  \frac{\sqrt{T}}{\diffp} \right)^{2/3} \log d \right).
    \end{equation*}
    
    Let us now analyze privacy. The privacy follows the same steps as in the proof of~\cref{thm:ub-priv-DS} with two main differences. First, let $t=t_1$ be the time such that $\tilde \ell_{t_1}$ contains the differing loss function and let $\tilde \ell_{t} = \tilde \ell_{t}(x_{t-1})$ and $\tilde \ell'_{t} = \tilde \ell'_{t}(x_{t-1})$. Note that $|\tilde \ell_{t_1} - \tilde \ell'_{t_1}| \le 1/B$ thus we have that $Z_t$ and $Z'_t$ are $\eta/(Bp)$-indistiguishable since
     \begin{align*}
    \frac{P(Z'_t = 1)}{P(Z_t = 1)}
        & \le \frac{(1-p)(1-\eta)^{\tilde \ell'_{t-1}}}{(1-p)(1-\eta)^{\tilde \ell_{t-1}}} \\
        &  \le  (1-\eta)^{-|\tilde \ell_{t-1} - \tilde \ell'_{t-1}|} \\
        &  \le e^{2\eta/B}.
    \end{align*}
    Moreover, assuming w.l.o.g. that $\tilde \ell'_{t-1} \ge \tilde \ell_{t-1}$, we have
    \begin{align*}
    \frac{P(Z'_t = 0)}{P(Z_t = 0)}
        & \le \frac{p + (1-p)(1 - (1-\eta)^{\tilde \ell'_{t-1}})}{p + (1-p)(1 - (1-\eta)^{\tilde \ell_{t-1}}) } \\
        &  \le 1 + \frac{(1-p)|1 - (1-\eta)^{\tilde \ell'_{t-1} - \tilde \ell_{t-1}}|}{p + (1-p)(1 - (1-\eta)^{\tilde \ell_{t-1}}) } \\
        & \le 1 + \frac{|1 - (1-\eta)^{\tilde \ell'_{t-1} - \tilde \ell_{t-1}}|}{p} \\
        & \le 1 + \frac{|{\tilde \ell'_{t-1} - \tilde \ell_{t-1}}|}{p} \le e^{\eta/(Bp)}.
    \end{align*}
    The second difference in the privacy analysis is that the sensitivity of the score of the exponential mechanism is now $1/B$ hence $X_t$ and $X'_t$ are now $4\eta/B$-DP. This shows that  $W_t$  given $\{ W_\ell \}_{\ell=0}^{t-1}$ and $W'_t$  given $\{ W'_\ell \}_{\ell=0}^{t-1}$  are $\diffp_t$-indistinguishable where 
    \begin{equation*}
        \diffp_t = 
        \begin{cases}
             0  & \text{if } t < t_1 \\
             \eta/(Bp) & \text{if } t = t_1 \\
             \indic{\sum_{\ell=1}^{t-1} Y_\ell < K} 4 Y_t \eta/B &\text{if } t > t_1
        \end{cases}
    \end{equation*}
    The result then follows from advanced composition~\citep{DworkRo14}: the final privacy parameter is 
    \begin{align*}
    \diffp_f 
        & \le \frac{3}{2} \sum_{t=1}^T \diffp_t^2 + \sqrt{6 \sum_{t=1}^T \diffp_t^2 \log(1/\delta) } \\
        & \le \frac{3}{2} (\frac{\eta}{Bp} + 16K \eta^2/B^2) + \sqrt{6(\frac{\eta^2}{B^2p^2} + 16K \eta^2/B^2)\log(1/\delta)  } \\
        & \le  \frac{5\eta}{Bp} + 24 K \eta^2/B^2 + \frac{10\eta}{B} \sqrt{K \log(1/\delta)} \\
         & \le  \frac{5\eta}{Bp} + 100 T p  \eta^2/B^3 + \frac{20\eta}{B} \sqrt{12 T p/B \log(1/\delta)}.
    \end{align*}

\section{Proofs for~\cref{sec:ub-stoch}}
\label{sec:apdx-ub-stoch}

\subsection{Proof of~\cref{thm:ub-stoch-OCO}}
\label{sec:thm-ub-stoch-OCO}
The privacy claim is immediate as each sample $\ell_i$ is used only once in running a single \ed-DP algorithm. Now we prove the claim about utility. Consider time-step $t=2^i$ where we invoke a DP-SCO algorithm with $t/2 = 2^{i-1}$ samples. 
Therefore the guarantees of the algorithm imply that at iteration $t$ we have
\begin{equation*}
        \E_{\ell_t \sim P} \left[\ell_t(x_t) - \min_{x \in [d]} \ell_t(x) \right] \le O \left( \Delta_{2^i} \right).
\end{equation*}
Therefore at phase $i$, that is $2^{i} \le t \le 2^{i+1}$, the total regret is at most 
\begin{equation*}
    \E\left[ \sum_{t=2^{i}}^{2^{i+1}}\ell_t(x_t) - \min_{x \in [d]} \sum_{t=2^{i}}^{2^{i+1}} \ell_t(x) \right] 
        \le O \left(2^i \Delta_{2^i} \right).
\end{equation*}
Summing over $i$ proves the claim.

\subsection{Proof of~\cref{cor:DP-exp-stoch}}
\label{sec:apdx-cor-DP-exp-stoch}
The algorithm $\Aone$ is $\diffp$-DP and has excess population loss $\Delta_n = O(\sqrt{\log(d)/n} + \log(d)/n\diffp)$~\cite[Theorem 6]{AsiFeKoTa21}. Thus, \cref{thm:ub-stoch-OCO} implies that 
\begin{align*}
     \E\left[ \sum_{t=1}^T \ell_t(x_t) - \min_{x \in [d]} \sum_{t=1}^T \ell_t(x) \right]
        & \le \sum_{i=1}^{\log T} 2^i \Delta_i \\
        & \le O \left( \sum_{i=1}^{\log T} 2^{i/2} \sqrt{\log(d)} + \log(d)/\diffp \right) \\
        & \le O \left( \sqrt{T \log(d)} + \log(d) \log(T)/\diffp \right). 
\end{align*}
