# Supplementary material for: Near-Optimal Algorithms for Private Online Optimization in the Realizable Regime
Source: arXiv:2302.14154 source file (2023-02-27)
Supplement: Supplementary file 4 [file appendix-realizable.tex]

%\section{Proofs for~\cref{sec:upper-bounds-realizable}}

% \subsection{Proof for~\cref{thm:ub-realizable-alt}}
% \label{sec:proof-realizable-binary-tree}
% \hac{complete this proof}

% Main idea for analysis: it is enough to show that $k= O(\log d)$ as this gives the claim. To this end, note that the adversary has to reduce the number of good experts by half to eliminate all experts in $S_k$.

% \subsection{Proof for~\cref{thm:ub-adaptive}}
% \label{sec:proof-thm-ub-adaptive}
% \hac{complete this}
