# Supplementary material for: Near-Optimal Algorithms for Private Online Optimization in the Realizable Regime
Source: arXiv:2302.14154 source file (2023-02-27)
Supplement: Supplementary file 7 [file realizable-appendix-potential.tex]

\section{Additional details for~\Cref{sec:alg-pot}}
\label{sec:apds-alg-pot}

We can obtain the following regret bounds for $\diffp$-DP using \cref{alg:potential-experts}.
\begin{theorem}(pure DP)
    Suppose that we run \cref{alg:potential-experts} with parameters $\alpha = 1$, $\beta = \frac{1}{T^2}$,  $K=2 \log 1/\gamma$ , $\diffp_0 = \diffp / K$, and $\eta =\diffp_0 / (56 \log T) = \diffp / (112 \log T \log 1/\gamma)$. If $L^*(\gamma) \leq \log^2 1/\gamma \log T / \diffp$, then this algorithm satisfies $\eps$-DP and incurs loss $O(L^* + \frac{\log^2 1/\gamma\log T}{\diffp}$. In particular, for DP-OPE with $d$ experts, assuming that that $OPT \leq \log^2 d \log T / \diffp$, we get regret  $O(\log^2 d \log T / \diffp)$ by setting $\gamma = \frac 1 d$.
\end{theorem}
